# Supplementary material for: Two-dimensional phosphorus carbide: Competition between sp2 and sp3 bonding
Source: arXiv:1604.05686 source file (2016-04-19)
Supplement: Supplementary file 1 [file 20160415-2D-PC16-SI.pdf]

# Supporting Information for: Two-dimensional phosphorus carbide: Competition between $sp^2$ and $sp^3$ bonding

Jie Guan,<sup>†</sup> Dan Liu,<sup>†</sup> Zhen Zhu,<sup>†,‡</sup> and David Tománek<sup>\*,†</sup>

<sup>†</sup>*Physics and Astronomy Department, Michigan State University, East Lansing, Michigan 48824, USA*

<sup>‡</sup>*Materials Department, University of California, Santa Barbara, California 93106, USA*

E-mail: tomanek@pa.msu.edu

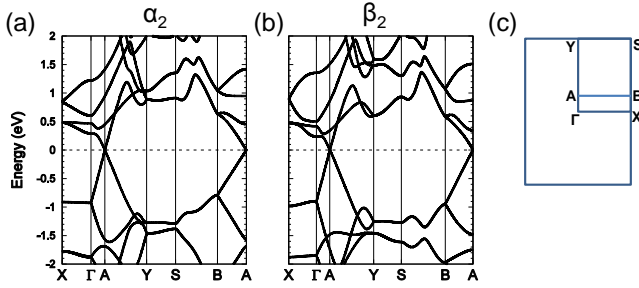

Figure S1: Band structure of semi-metallic (a)  $\alpha_2$ -PC and (b)  $\beta_2$ -PC near the Dirac point. (c) Definition of the high-symmetry points in the Brillouin zone of the structures in (a) and (b).

## Band structure near the Dirac point of $\alpha_2$ -PC and $\beta_2$ -PC

The band structure of semi-metallic  $\alpha_2$  and  $\beta_2$  allotropes of PC, described in the main manuscript, is displayed in Figure S1(a) and S1(b). Each structure has a Dirac point at point A located in-between  $\Gamma$  and Y in the Brillouin zone shown in Figure S1(c). The unusual location of the Dirac points inside the Brillouin zone differs from its location in Brillouin zone corners in graphene. Due to the strong structural anisotropy in the systems, the Dirac cone is anisotropic and thus not a true cone. The opening angle of the cone, given by the  $E(\mathbf{k})$  dispersion near A, is largest along the A – B direction and the smallest along the A –  $\Gamma$  or

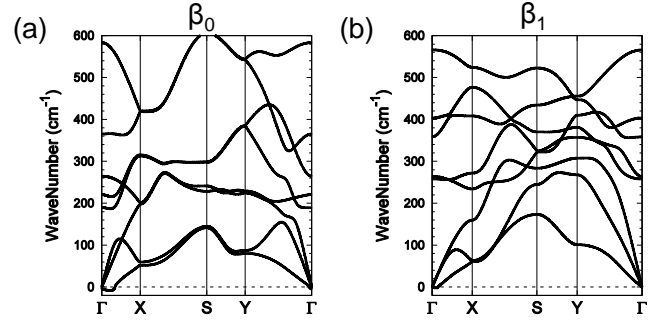

Figure S2: Phonon spectra of (a)  $\beta_0$ -PC and (b)  $\beta_1$ -PC monolayers.

A – Y direction. We have found that uniaxial strain may be used to eliminate the anisotropy of the Dirac cone. At the same time, however, also the location of the Dirac point along  $\Gamma$  – Y line in the Brillouin zone changes.

## Stability and vibration spectra of selected PC monolayers

We found all structures discussed in the main manuscript to be stable not only in terms of their large cohesive energy, but also resistant under arbitrary deformations. The latter point can be validated by showing that the phonon spectra of unsupported monolayers are free of imaginary frequencies that would indicate spontaneous collapse of the structure in a way dictated by the particular soft mode character. Computation of phonon spectra of 2D structures with a low flexural rigidity is very de-

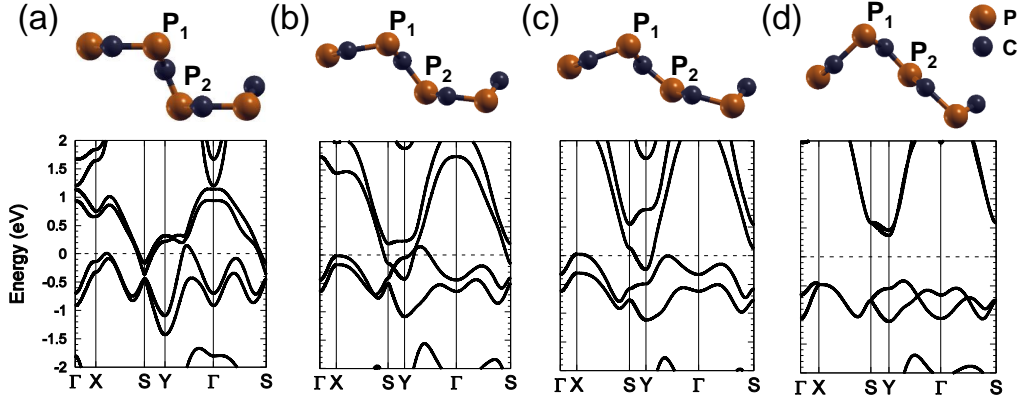

Figure S3: (Color online) Spontaneous structural transformation of  $\alpha_0$ -PC from its initial armchair profile in (a) to the final structure with a zigzag profile in (d). Snap shots of the intermediate structures, shown in side view in the upper panels, are accompanied by the corresponding band structure in the lower panels. Noteworthy is the transition from a metallic structure in (a) to a semiconductor in (d). The significance of the inequivalent  $P_1$  and  $P_2$  sites is discussed in the main text.

manding, since such calculations require very large supercells to yield converged results in particular for the flexural  $Z$  mode with an  $\omega(k) \propto k^2$  dispersion near the  $\Gamma$  point. For the sake of illustration, we present the phonon spectra of  $\beta_0$ -PC and  $\beta_1$ -PC monolayers in Figure S2. The soft out-of-plane acoustic  $Z$  modes can be clearly distinguished from the in-plane transverse acoustic and the in-plane longitudinal acoustic modes, which are the hardest of the three. Clearly, further structural stabilization that suppresses the  $Z$  modes will occur when PC is deposited on a substrate.

### Structural transformation in $\alpha_0$ -PC

As discussed in the main manuscript,  $\alpha$  allotropes are generally distinguished by their armchair profile reminiscent of black phosphorus.<sup>1</sup> This is true for  $\alpha_1$ -PC and  $\alpha_2$ -PC, but does not hold for  $\alpha_0$ -PC, which spontaneously reconstructs to a zigzag profile.

To make sure that the reconstruction process of  $\alpha_0$ -PC is unique and that all structures discussed in this manuscript represent the true equilibrium configuration, which is not an artifact of unit cell limitations, we have doubled the unit cells of all allotropes and found no further changes.

The reconstruction process of  $\alpha_0$ -PC can be seen in the accompanying movie

`alpha0-optimization.avi` with snap shots of the process shown in the upper panels of Figure S3(a)-S3(d). The changing band structure, calculated using the DFT-PBE functional, is presented below the structural snap shots in Figure S3. These results allow to follow the gradual transitions from the initial metallic structure in (a) to a semiconductor with a 0.7 eV wide band gap in (d). The band gap opening comes along with a symmetry reduction, best seen in the transformation of the local environment at the  $P_1$  and  $P_2$  sites, which were equivalent in (a) and become significantly different in (d).

### Dependence of the electronic structure of PC monolayers on the exchange-correlation functional

It is well known that the fundamental band gap is usually underestimated in DFT-PBE calculations. The proper way to determine the electronic band structure involves computationally much more demanding self-energy calculations, often performed using the GW approximation.<sup>2,3</sup> Calculations using a hybrid exchange-correlation functional such as HSE06<sup>4,5</sup> are computationally less involved and may reproduce the observed fundamental band gap correctly, but the results depend on the mixing of Hartree-Fock and DFT-PBE functionals. We

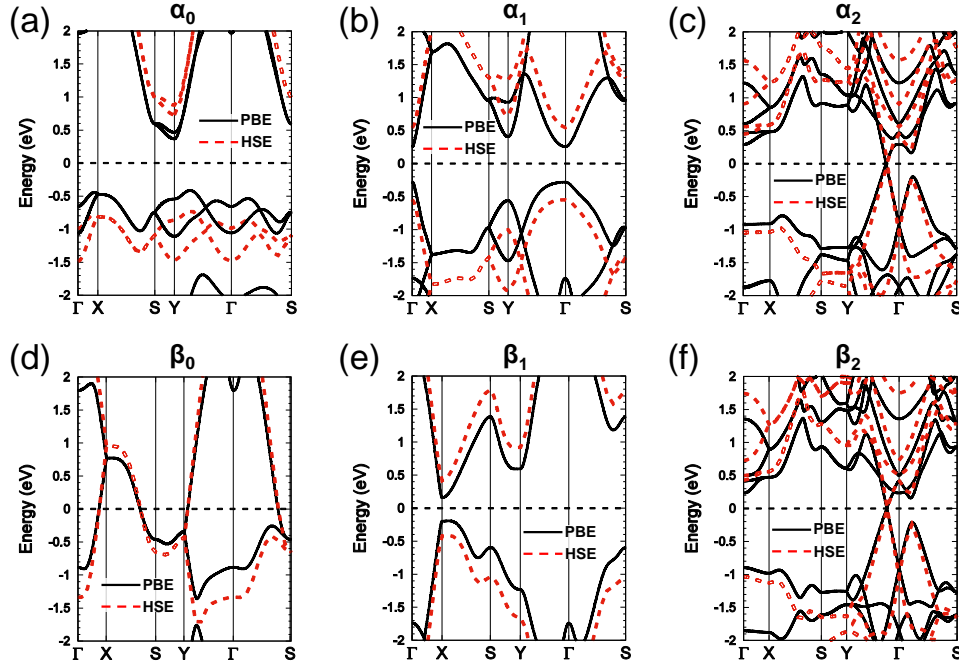

Figure S4: (Color online) Electronic band structure of (a)  $\alpha_0$ -PC, (b)  $\alpha_1$ -PC, (c)  $\alpha_2$ -PC, (d)  $\beta_0$ -PC, (e)  $\beta_1$ -PC, (f)  $\beta_2$ -PC monolayer obtained using DFT calculations with PBE and HSE06 exchange-correlation functionals.

compare the electronic band structure of the six PC monolayer structures discussed in the main manuscript, calculated by DFT-PBE and HSE06, in Figure S4. Our HSE06 studies use the default value of 0.25 for the mixing parameter and, for the sake of fair comparison, the identical geometry that had been optimized by DFT-PBE.

Band structure results in Figure S4 indicate that for the semiconducting  $\alpha_0$ -PC,  $\alpha_1$ -PC and  $\beta_1$ -PC structures, HSE06 shifts occupied states rigidly down and unoccupied states up with respect to the Fermi level, thus increasing the band gap value. As a result, HSE06 gives band gap values of 1.5 eV for  $\alpha_0$ -PC, 1.1 eV for  $\alpha_1$ -PC, and 0.8 eV for  $\beta_1$ -PC. As a consequence of the increased band gap, the compressive in-layer strain required to close this gap in  $\alpha_1$ -PC and  $\beta_1$ -PC will be larger than what was expected based on DFT-PBE results. HSE06 does not affect the metallic character of  $\beta_0$ -PC and semi-metallic character of  $\alpha_2$ -PC and  $\beta_2$ -PC predicted by DFT-PBE, but increases the band dispersion and thus the width of the valence and conduction bands.

## References

- (1) Guan, J.; Zhu, Z.; Tománek, D. *Phys. Rev. Lett.* **2014**, *113*, 046804.
- (2) Hybertsen, M. S.; Louie, S. G. *Phys. Rev. B* **1986**, *34*, 5390–5413.
- (3) Deslippe, J.; Samsonidze, G.; Strubbe, D. A.; Jain, M.; Cohen, M. L.; Louie, S. G. *Comp. Phys. Commun.* **2012**, *183*, 1269–1289.
- (4) Heyd, J.; Scuseria, G. E.; Ernzerhof, M. *J. Chem. Phys.* **2003**, *118*, 8207–8215.
- (5) Krukau, A. V.; Vydrov, O. A.; Izmaylov, A. F.; Scuseria, G. E. *J. Chem. Phys.* **2006**, *125*, 224106.
